# Supplementary material for: Constructing and Analyzing the LSM Compaction Design Space (Updated Version)
Source: arXiv:2202.04522 source file (2022-02-26)
Supplement: Supplementary file 1 [file 9-appendix.tex]

\red{Trying out alternate organization. We need to define each of the performance metrics before, if we choose to adopt this format.}
 
\subsection*{4.1* Compaction Eagerness}
Below, we discuss how the performance of an LSM-based storage engine is affected by the compaction eagerness. 

\Paragraph{Leveling} A leveled LSM-tree eagerly merges the overlapping sorted runs every time a level is saturated and affects the performance the storage engine as follows.

\textit{Write amplification}: In a leveled LSM-tree, every time a Level $i$ reaches its capacity, all (or a subset of) files from Level $i$ are compacted with all (or the overlapping) the files from Level $i+1$; thus, on average each entry is written $T$ times within a level which leads to an average-case write amplification of $\mathcal{O}(T \cdot L)$. 

\textit{Write throughput}: A leveled LSM-tree performs compactions eagerly whenever the memory buffer is full or a disk level reaches a nominal capacity. 
This triggers compactions frequently, which consumes the device bandwidth at a greater degree, and affects the write throughput adversely. 

\textit{Point lookups}: For leveling, the average cost for a point lookup on an non-existing key is given as $\mathcal{O}(L \cdot e^{-BPK})$, and that on an existing key is $\mathcal{O}(1 + L \cdot e^{-BPK})$ as it must always perform at least one I/O to fetch the target key.

\textit{Range lookups}: Compaction eagerness controls the number of sorted runs in an LSM-tree, and therefore, influences the cost for range lookups. 
The average cost for a long range lookup is given as $\mathcal{O}(\tfrac{s \cdot N}{B})$ for leveling, with $s$ being the average selectivity of the range queries. 
For short range queries, the average cost is simply proportional to the number of sorted runs, and is given as $\mathcal{O}(L)$.

\textit{Space amplification}: In presence of only updates and no deletes in a workload, the worst-case space amplification in a leveled LSM-tree is $\mathcal{O}(1/T)$~\cite{Dayan2018}. 
However, with the addition of deletes, the space amplification increases significantly, and is given as $\mathcal{O}(\tfrac{N}{1 - \lambda})$ for leveling, where $\lambda$ is ratio of the size of a tombstone and the average size of a key-value pair~\cite{Sarkar2020}. 
The space amplification for hybrid designs lay between the two extremely, and depends heavily on the exact tree design. 

\textit{Delete performance}: The average time taken to persistently delete an entry from a tree is given by $\mathcal{O}(\tfrac{T^{L-1} \cdot P \cdot B}{I})$ for leveling~\cite{Sarkar2020}, where $I$ denotes the rate of ingestion of unique entries to the database. 
Note that, for leveling propelling the tombstone to the last level ensures persistent deletion of the target entry to guarantee delete persistence. 

\Paragraph{Tiering}: A tiered LSM merger the sorted runs lazily and is optimized for writes.

\textit{Write amplification}: For a tiered LSM, each level may have up to $T$ sorted runs with overlapping key-ranges; thus, each entry is written at least once per level resulting in an average-case write amplification of $\mathcal{O}(L)$. 

\textit{Write throughput}: For tiering, compactions are less frequent and with the device bandwidth mostly free of compaction traffic, the write throughput is significantly improved. 

\textit{Point lookups}: The average point lookup cost for a tiered LSM is $\mathcal{O}(T \cdot L \cdot e^{-BPK})$ for lookups on an non-existing key, and $\mathcal{O}(1 + T \cdot L \cdot e^{-BPK})$ for existing keys. 

\textit{Range lookups}: For tiering, the average cost for a long range lookup is given as $\mathcal{O}(\tfrac{T \cdot s \cdot N}{B})$, and that for short range lookups is $\mathcal{O}(T \cdot L)$ for tiering. 

\textit{Space amplification}: The worst-case space amplification in a leveled LSM-tree is $\mathcal{O}(T)$~\cite{Dayan2018} for workloads with updates but no deletes; which increases to $\mathcal{O}(\tfrac{(1 - \lambda) \cdot N + 1}{\lambda \cdot T})$ in presence of deletes.

\textit{Delete performance}: The average latency for delete persistence for a tiered LSM is given by $\mathcal{O}(\tfrac{T^L \cdot P \cdot B}{I})$, as in case of tiering, the tombstone must participate in a compaction involving all the sorted runs from the last level to guarantee delete persistence. 

\Paragraph{Hybrid Designs}: Hybrid LSM-designs are generalized by $l$-leveling which includes lazy leveling, RocksDB-style hybrid leveling with only the first level being tiered, and other LSM-variants proposed in \cite{Dayan2019} and \cite{Idreos2019}.

\textit{Write amplification}: An $l$-leveled LSM-tree has its last $l$ levels implemented as leveled with the remaining shallower $L-l$ levels as tiering; and thus, the average-case write amplification in an $l$-leveled tree is given as $\mathcal{O}(L-l) + \mathcal{O}(T \cdot l)$. 
For lazy leveling, $l = 1$, which asymptotically makes the write amplification of the LSM-tree similar an tiered LSM; while for RocksDB-style hybrid leveling $l = L-1$ closely resembles the write amplification of a leveled LSM.
% Similarly, for a hybrid LSM-tree, the average-case write amplification can be expressed as $\mathcal{O}(L-i) + \mathcal{O}(T \cdot i)$, where $L-i$ denotes the number of tiered levels in the tree. 

\textit{Write throughput}: The write throughput of hybrid LSM-designs fall in between that of leveling and tiering, and depends on the capacity of the number of leveling implemented as tiering or leveling.

\textit{Point lookups}: For a hybrid design, the average lookup cost for non-existing keys becomes \red{fill in}, and similarly for lookups on existing keys. 

\textit{Range lookups}: For hybrid designs, the cost for range lookups fall in between that for leveling and tiering, and depends on the exact design of the tree. 

\textit{Space amplification}: The space amplification for hybrid designs lay between the two extremely, and depends heavily on the exact tree design. 

\textit{Delete performance}: The hybrid designs, the latency to persist deletes depends only on the implementation of the last level of the tree, i.e., if the last level is implemented as tiered, the said latency is same as a tiered LSM; otherwise, which is similar to a leveled LSM-tree.

\begin{table*}[t] 
    \centering
    \resizebox{\textwidth}{!}{%
        \begin{tabular}{l|l}
        \toprule
        \multirow{1}{*}{\textbf{Knobs}}  & \textbf{Remark} \\
        \midrule
        \multirow{1}{*}{Size ratio}  & \shortstack[l]{
            \textit{Space-amplification}: Larger size ratio → fewer levels → reduce space-amp  \\ 
            \textit{Write-amplification}: Larger size ratio → more times that an entry averagely gets merged → increase write amplification. \\ 
            \textit{Update cost}: Larger size ratio → more times that an update entry averagely gets merged till it consolidates → more average worst-case update cost \\
            \textit{Read cost}: Larger size ratio → fewer levels → fewer expected lookup cost O(L). \\
            \textit{Individual compaction bytes}: Larger size ratio → more entries to be copied during a compaction → more total compaction bytes. \\
            \textit{*Update throughput}: ? \\
            \textit{Modeling graph: https://www.desmos.com/calculator/q4ko9j1wmp}
            } \\ 
        \midrule
        \multirow{1}{*}{Memory buffer}  & \shortstack[l]{
            \textit{Space-amplification}: Larger memory buffer → fewer levels → reduce space-amp in general and can be slightly optimized for skewed workloads.  \\ 
            \textit{Write-amplification}: Larger memory buffer → every entry participates in averagely the same number of compaction in total → No changes. \\ 
            \textit{Update cost}: Larger memory buffer → fewer levels → an updating entry participates in a fewer numbers of compactions in total to consolidate → less average worst-case update cost \\
            \textit{Read cost}: Larger memory buffer → fewer levels → fewer expected lookup cost O(L). \\
            \textit{Individual compaction bytes}: Larger memory buffer → Larger file size → more entries to be copied during a compaction → more individual compaction bytes. \\
            \textit{*Read throughput}: ? \\
            \textit{*Update throughput}: ? \\
            \textit{Modeling graph: https://www.desmos.com/calculator/udmwdg5dt1}
            } \\ 
        \midrule
        \multirow{1}{*}{File size}  & \shortstack[l]{
            \textit{Space-amplification}: No changes. \\ 
            \textit{Write-amplification}: No changes. \\ 
            \textit{Update cost}: No changes. \\
            \textit{Read cost}: No changes. \\
            \textit{Individual compaction bytes}: Larger file size → more entries to be copied during a compaction → more individual compaction bytes \\
            \textit{*Read throughput}: ? \\
            \textit{*Update throughput}: ? \\
            \textit{Others}:
            } \\ 
        \midrule
        \multirow{1}{*}{Bloom filters}  & \shortstack[l]{
            \textit{Space-amplification}: Larger bytes per key → increase space-amplification. \\ 
            \textit{Write-amplification}: No changes. \\ 
            \textit{Update cost}: No changes. \\
            \textit{Read cost}: Larger bytes per key → assume more memory allocated to Bloom filter → fewer read cost O(L) \\
            \textit{Individual compaction bytes}:  Larger bytes per key → more bytes written in individual compactions. \\
            \textit{*Read throughput}: ? \\
            \textit{*Update throughput}: ? \\
            \textit{Others}:
            } \\ 
        \midrule
        \multirow{1}{*}{Block cache}  & \shortstack[l]{
            \textit{Space-amplification}: No changes. \\ 
            \textit{Write-amplification}: No changes. \\ 
            \textit{Update cost}: No changes. \\
            \textit{Read cost}:  Cache indexes, filters, data blocks for reads → significantly better read performance. \\
            \textit{Read throughput}: Directly read from memory → significantly larger read throughput. \\
            \textit{Individual compaction bytes}: No changes.\\
            \textit{*Update throughput}: ? \\
            \textit{Others}: Reads are more optimized for skewed workloads.
            } \\
        \midrule
        \multirow{1}{*}{Threads}  & \shortstack[l]{
            \textit{Space-amplification}: No changes. \\ 
            \textit{Write-amplification}: No changes. \\ 
            \textit{Update cost}: No changes. \\
            \textit{Read cost}: Shorten compaction duration → Timely reclamation that can potentially reduce read amplification if a bunch of reads is right after multi-level-compactions that are triggered by intensive updates. \\
            \textit{Individual compaction bytes}: No changes. \\
            \textit{Read throughput}: Shorten compaction duration → increase read throughput for interleaved workloads.\\
            \textit{Update throughput}: Shorten compaction duration → increase overall write throughput. \\
            \textit{*Others}: Shorten compaction duration → consolidate duplicate and discarded entries timely → reduce read amplification and  lookup cost → and better space amplification?
            } \\ 
        \midrule
        \multirow{1}{*}{File size multiplier}  & \shortstack[l]{
            \textit{Space-amplification}: No changes. \\ 
            \textit{Write-amplification}: Larger file size multiplier → larger level contributes to a larger number of entries copied during a compaction with the same compaction frequency → increase write-amplification. \\ 
            \textit{Update cost}: Larger file size multiplier → larger level contributes to a larger number of entries copied during a compaction with the same compaction frequency → more update cost. \\
            \textit{Read cost}: No changes.  \\
            \textit{Individual compaction bytes}: Larger file size multiplier → larger level has larger compaction bytes but with the same compaction frequency.  \\
            \textit{Read throughput}: No changes. \\
            \textit{Update throughput}: Shorten compaction duration → increase overall write throughput. \\
            \textit{Others}:
            } \\ 
        \midrule
        \multirow{1}{*}{Level$_0$ compaction trigger}  & \shortstack[l]{
            \textit{Space-amplification}: More Level$_0$ files → increase space-amplification. \\ 
            \textit{Write-amplification}: Level$_0$ self compactions → increase write-amplification.  \\ 
            \textit{Update cost}: More Level$_0$ files → more times of compactions to consolidates a existing entry. \\
            \textit{Read cost}: More Level$_0$ files → increase space-amplification and read amplification → higher read cost. \\
            \textit{Individual compaction bytes}: More compaction bytes between Level$_0$ and Level$_1$ compactions.\\
            \textit{Update throughput}: More Level$_0$ files → increase insert/update throughput. \\
            \textit{*Read throughput}: ? \\
            \textit{Others}:
            } \\
        \midrule
        \multirow{1}{*}{Max compaction bytes}  & \shortstack[l]{
            \textit{Space-amplification}: If too small, redundant entries might not be compacted in a timely manner → increase space-amplification. \\ 
            \textit{*Write-amplification}: ? \\ 
            \textit{*Update cost}: ? \\
            \textit{Read cost}: If too small, redundant entries might not be reclaimed in time → increase read cost. \\
            \textit{*Read throughput}: ? \\
            \textit{Individual compaction bytes}: No changes.\\
            \textit{Update throughput}: If too small, further compactions needed to be done → reduce update throughput.  \\
            \textit{Others}:
            } \\
        \midrule
        \multirow{1}{*}{Compaction readahead size}  & \shortstack[l]{
            \textit{Space-amplification}: No changes. \\ 
            \textit{Write-amplification}: No changes. \\ 
            \textit{Update cost}: No changes. \\
            \textit{Read cost}: Perform bigger reads when doing compactions → increase read amplification and read cost. \\
            \textit{*Read throughput}: ? \\
            \textit{Individual compaction bytes}: No changes.\\
            \textit{Update throughput}: No changes. \\
            \textit{Others}: 
            } \\
        \bottomrule
        \end{tabular}
    }
    \caption{LSM-Tree compaction tuning knobs. \label{tab:cost}}
    \vspace{-0.2in}
\end{table*}
